# Supplementary material for: Robotic Perception of Object Properties using Tactile Sensing
Source: arXiv:2112.14119 source file (2021-12-28)
Supplement: Supplementary file 1 [file appendix01.tex]

\begin{frontmatter}
\chapter{Appendix title}%\label{chap:appa}
\end{frontmatter}

%\section{}\label{}
